# Supplementary material for: Magnetoelasticity of $\mathrm{Co_{25}}\mathrm{Fe_{75}}$ thin films
Source: arXiv:1906.05543 ancillary file (2019-06-13)
Supplement: Supplementary file 1 [file Supplementary.pdf]

# Supplemental information: Magnetoelasticity of CoFe thin films

Daniel Schwienbacher,[1,2,3,4,*] Matthias Pernpeintner,[1,2,3] Lukas Liensberger,[1,2] Eric R.J.Edwards,[5] Hans T. Nembach,[5] Justin M. Shaw,[5] Mathias Weiler,[1,2] Rudolf Gross,[1,2,3,4] and Hans Huebl[1,2,3,4,†]

[1] *Walther-Meissner-Institut, Bayerische Akademie der Wissenschaften, Walther Meissner Str.8 85748 Garching*

[2] *Technische Universität München, James-Franck-Str. 1, 85748 Garching, Germany*

[3] *Nanosystems Initiative Munich, Schellingstraße 4, 80799 München, Germany*

[4] *Munich Quantum Center, Hans-Kopfermann-Str. 1, 85748 Garching, Germany*

[5] *National Institute of Standards and Technology, Boulder, Colorado 80305, USA*

(Dated: May 27, 2019)

* daniel.schwienbacher@wmi.badw.de

† hans.huebl@wmi.badw.de;

## I. DERIVATION OF THE RESONANCE FREQUENCY OF A TENSILE STRESSED STRING RESONATOR CONSIDERING THE BENDING AT THE CLAMPS

The resonance frequency of a highly tensile stressed string (HTS) resonator is given by [1, 2]

$$\Omega_{n,\mathrm{HTS}} = \frac{n\pi}{L}\sqrt{\frac{\sigma_0}{\rho}}, \tag{1}$$

where $n$ is the mode index, $L$ is the length of the string, $\sigma_0$ is the tensile stress of the material and $\rho$ its density. This formula assumes that the additional energy due to a displacement is only stored in the stress of the string, i.e. it neglects the bending of the material and the stored energy. In the following we discuss the effect of bending on the resonance frequency of the string to first order. The derivation follows the discussion in Ref. [3].

We start using the Euler-Bernoulli beam theory for a pre-stressed prismatic beam with cross-section $A = wt$, where $w$ is the string's width and $t$ its thickness. Considering a restoring force based on the bending of the string and the change in the stress $\mathrm{d}F_{\mathrm{restoring}} = \mathrm{d}F_{\mathrm{bending}} + \mathrm{d}F_{\mathrm{prestress}}$, we obtain the equation of motion for the transverse vibrational mode of the an infinitesimal volume element of the beam [4, 5]:

$$-EI\frac{\partial^4 v}{\partial x^4} + \sigma_0 A\frac{\partial^2 v}{\partial x^2} = \rho A\frac{\partial^2 v}{\partial t^2}, \tag{2}$$

with $EI$ being the flexural rigidity composed of the Young's modulus $E$ and the moment of inertia $I$. If we assume a harmonic time dependence for the local displacement $v(x,t) = v(x)\exp(-i\Omega t)$[4] the differential equation transforms to:

$$-EIv^{(4)}(x) + \sigma_0 A v^{(2)}(x) = -\rho A\Omega^2 v(x) \tag{3}$$

The general solution for Eq. (3) is given by [4, 5]

$$v(x) = c_1\exp(\alpha x) + c_2\exp(-\alpha x) + c_3\sin(\beta x) + c_4\cos(-\beta x) \tag{4}$$

with

$$\alpha = \sqrt{\mu_+} > 0, \text{and} \tag{5}$$

$$\beta = -i\sqrt{\mu_-} > 0. \tag{6}$$

$$I = \frac{wt^3}{12}, \tag{7}$$

$$A = wt, \tag{8}$$

$$\mu_\pm = \frac{\sigma_0 A \pm \sqrt{\sigma_0^2 A^2 + EI\rho A\Omega^2}}{2EI}, \tag{9}$$

For a doubly clamped beam the boundary conditions are given by [4, 5]:

$$v(x = \pm L/2) = 0 \tag{10}$$
$$\partial v(x = \pm L/2)/\partial x = 0$$

The application of these boundary conditions to the general solution (4) results in a homogeneous system of four linear equations and four variables $c_i\,(i = 1, 2, 3, 4)$. Non trivial solutions for the displacement are given by a vanishing determinant of this system:

$$e^{-\alpha L}\left[\left(\alpha^2 - \beta^2\right)\left(e^{2\alpha L} - 1\right)\sin(\beta L) + 4\alpha\beta/(e^{2\alpha L} + 1)\cos(\beta L)\right] = 0 \tag{11}$$

While the above result is general, we want to focus next on suitable approximations for our problem. For our tensile stressed (TS) nano-strings, $4EI\rho A\Omega^2 \ll \sigma_0^2 A^2$. In this case, we can expand the square root in (9) to first order

$$\mu_\pm \approx \frac{\sigma_0 A}{2EI}\left[1 \pm \left(1 + \frac{2EI\rho A\Omega^2}{\sigma_0^2 A^2}\right)\right]. \tag{12}$$

Combining (12) with (5) and (9) we obtain

$$\alpha \approx \alpha_0 := \sqrt{\frac{\sigma_0 A}{EI}} \text{ and} \tag{13}$$
$$\beta \approx \sqrt{\frac{\rho}{\sigma_0}}\Omega. \tag{14}$$

Next we substitute the HTS approximation Eq. (1) into Eq. (14) and obtain

$$\beta L = \sqrt{\frac{\rho}{\sigma_0}}\Omega_{n,\mathrm{HTS}}L \approx \pi n. \tag{15}$$

Therefore,

$$\cos(\beta L) \approx (-1)^n.$$

This simplifies Eq. (11) to

$$\left(\alpha_0^2 - \beta^2\right)\left(e^{2\alpha_0 L} - 1\right)\sin(\beta L) + 2\alpha_0\beta\left[2e^{\alpha_0 L} - (-1)^n e^{2\alpha_0 L} + (-1)^n\right] = 0. \tag{16}$$

For the geometries discussed in this work, which are $L \approx 50\,\mu\mathrm{m}$, $t \approx w \approx 100\,\mathrm{nm}$ (see also Sec. III) and material parameters [2, 6], we find $\alpha_0 > 10\beta$ with $\beta L \approx n\pi > 1$. Thus $e^{\alpha_0 L} \gg 1$. Under these conditions, (16) reduces to

$$(\alpha_0^2 - \beta^2)\sin(\beta L) - (-1)^n 2\alpha_0\beta = 0.$$

Using $\alpha_0 \gg \beta$ we obtain

$$\alpha_0 \sin(\beta L) - (-1)^n 2\beta = 0. \tag{17}$$

Next, we solve for $\beta$ by using (15) and expanding $\sin(\beta L)$ around $n\pi$:

$$\sin(\beta L) \approx (-1)^n (\beta L - n\pi). \tag{18}$$

Substituting this into Eq. (17), we obtain

$$\beta = \frac{n\alpha_0 \pi}{\alpha_0 L - 2}. \tag{19}$$

As last step we identify $\alpha_0$ and $\beta$ using Eqs. (13) and (14) with the geometry parameters of the resonator and the resonance frequency $\Omega_n/2\pi$. We obtain

$$\Omega_{n,\mathrm{TS}} = \frac{n\sigma_0 \pi \sqrt{A/\rho}}{\sqrt{\sigma_0 A}L - 2\sqrt{EI}} = \Omega_{n,\mathrm{HTS}} \frac{\sqrt{\sigma_0 A}L}{\sqrt{\sigma_0 A}L - 2\sqrt{EI}}. \tag{20}$$

Equation (20) represents the first oder correction accounting for the bending of the resonator. To further include the impact of the magnetoelasticity on the resonance frequency of the system, we adapt this formula using the replacements

$$\rho \to \rho_{\mathrm{eff}} \tag{21}$$

$$\sigma_0 \to \sigma_0 + \sigma_1 \cos(\Theta)^2. \tag{22}$$

The stress in the CoFe is separated into a magnetostrictive component $\sigma_{\mathrm{CoFe,mag}} := \sigma_1 \cos(\Theta)^2$ depending on the magnetization direction and a static contribution $\sigma_{\mathrm{CoFe,stat}}$ [2]. This static part contributes to the pre-stress in the string which is redefined as $\sigma_0 = \sigma_{\mathrm{string}} + \sigma_{\mathrm{CoFe,stat}}$. Using the moment of inertia of a string oscillating out of plane $I = wt^3/12$ [4] we obtain Eq. (1) in the main text

$$\Omega_{n,\mathrm{TS}} = \frac{n(\sigma_0 + \sigma_1 \cos(\Theta)^2)\pi \sqrt{\rho_{\mathrm{eff}}^{-}1}}{\sqrt{(\sigma_0 + \sigma_1 \cos(\Theta)^2)}L - 2\sqrt{Et^2/12}}, \tag{23}$$

which is used for the global fit discussed in Sec. (V).

## II. MAGNETIZATION DAMPING OF COFE STACKS ON SIN SUBSTRATES MEASURED USING BROADBAND MAGNETIC RESONANCE

We perform broadband ferromagnetic resonance measurements (bbFMR) to investigate the magnetization damping properties of extended CoFe thin films on reference SiN substrates at room temperature[7]. The continuous CoFe films were grown on $Si_3N_4$ (SiN) in

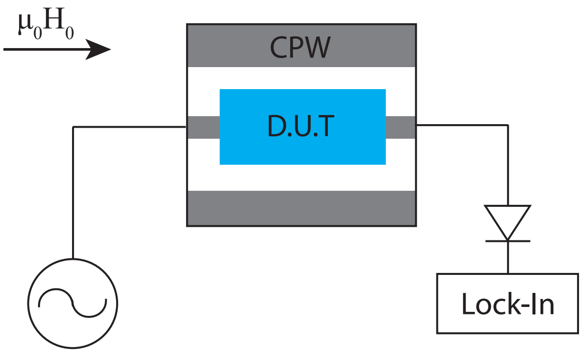


Figure 1. Sketch of the FMR measurement setup: The sample is positioned on a coplanar waveguides (CPW) center conductor with the CoFe facing the CPW. The CPW is connected to a microwave source on one side and to a microwave diode and a lock in amplifier at the other. An external magnetic field is applied in plane parallel to the CPW.

the same process as the string samples investigated in the main text. The bbFMR measurements were performed as described in Ref. [7, 8]. For the bbFMR, the CoFe layer faced the center conductor of the coplanar waveguide (center conductor width $\approx 250\,\mu\mathrm{m}$), which was located between the pole pieces of an electromagnet. A static magnetic field of $|\mu_0 H_0| \leq 1\,\mathrm{T}$ was applied parallel to the sample surface, along the center conductor. FMR spectra were acquired for various microwave frequencies $f \leq 43.5\,\mathrm{GHz}$ using a microwave diode detection scheme including a lock-in amplifier and microwace frequency modulation (c.f. Fig. 1). In a first step, we fit the FMR data (an example is shown in Fig. 2a)) to a Lorentzian lineshape to extract the resonance magnetic field $H_{\mathrm{res}}$ and linewidth $\Delta H$ for each frequency $f$. Fitting the resonance magnetic field $H_{\mathrm{res}}$ vs frequency $f$ (see Fig. 2 b)) to [7]

$$f(H_{\mathrm{res}}) = \frac{|\gamma|}{2\pi}\mu_0\sqrt{(H_{\mathrm{res}} + H_{\mathrm{aniso}})(H_{\mathrm{res}} + H_{\mathrm{aniso}} + M_{\mathrm{eff}})}, \tag{24}$$

yields the effective magnetization $M_{\mathrm{eff}}$, the in-plane anisotropy $H_{\mathrm{aniso}}$ and the gyromagnetic ratio $\gamma$. The Gilbert damping was extracted from the linewidth over frequency data (c.f. Fig. 2 c)) using [7]

$$\mu_0\Delta H = \mu_0\Delta H_0 + \frac{4\pi\alpha f}{|\gamma|}. \tag{25}$$

Here we obtain $\alpha = (4.2 \pm 0.2) \times 10^{-3}$ for a 20 nm thick $Co_{10}Fe_{90}$ film, which is in good agreement with the values measured by Schoen et al.[9].

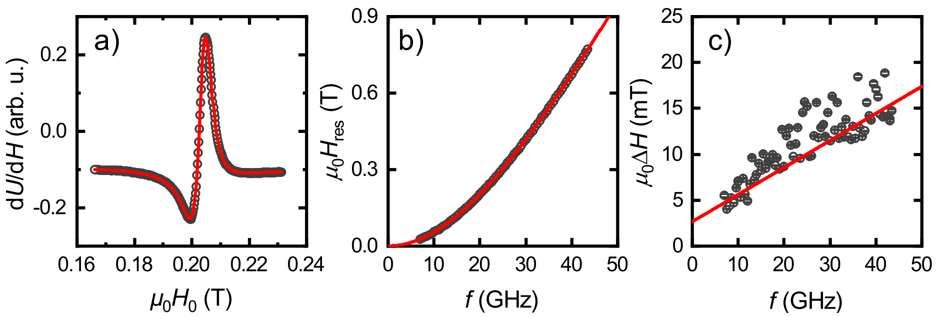


Figure 2. a) Field-swept FMR measurement at $f = 20\,\mathrm{GHz}$. Frequency dependence of the resonance field $H_{\mathrm{res}}$ b) and full with half maximum $\Delta H$ (c) of the FMR spectra obtained from 20 nm $Co_{10}Fe_{90}$ grown on top of a $Si_3N_4$ substrate. The solid lines are fits to the data.


[1] S. S. Verbridge, J. M. Parpia, R. B. Reichenbach, L. M. Bellan, and H. G. Craighead, Journal of Applied Physics **99**, 124304 (2006).

[2] M. Pernpeintner, R. B. Holländer, M. J. Seitner, E. M. Weig, R. Gross, S. T. B. Goennenwein, and H. Huebl, Journal of Applied Physics **119**, 093901 (2016).

[3] M. Pernpeintner, *Nanomechanical Hybrid Systems*, Ph.D. thesis, Technical University Munich (2016).

[4] S. Timoshenko, W. Weaver, and D. Young, *Vibration Problems in Engeneering* (John Wiley and Sons: New York, 1990 5th ed.).

[5] A. N. Cleland, *Foundations of nanomechanics: from solid-state theory to device applications* (Springer Science & Business Media, 2003).

[6] F. Cardarelli, in *Materials Handbook: A Concise Desktop Reference* (Springer International Publishing, 2018) pp. 101–248.

[7] S. S. Kalarickal, P. Krivosik, M. Wu, C. E. Patton, M. L. Schneider, P. Kabos, T. J. Silva, and J. P. Nibarger, Journal of Applied Physics **99**, 093909 (2006).

[8] R. Ohshima, S. Klingler, S. Dushenko, Y. Ando, M. Weiler, H. Huebl, T. Shinjo, S. T. Goennenwein, and M. Shiraishi, Applied Physics Letters **110**, 182402 (2017).

[9] M. A. W. Schoen, D. Thonig, M. L. Schneider, T. J. Silva, H. T. Nembach, O. Eriksson, O. Karis, and J. M. Shaw, Nat Phys **12**, 839 (2016).
